# Supplementary material for: Instance As Identity: A Generic Online Paradigm for Video Instance Segmentation
Source: arXiv:2208.03079 source file (2022-08-16)
Supplement: Supplementary file 1 [file 7-appendix.tex]

\section{Appendix}

\noindent\textbf{More Qualitative Results.}
In Fig.~\ref{fig:visualization} and Fig.~\ref{fig:visualization2}, we compare IAI predictions with MaskTrack R-CNN predictions. As the qualitative results show, our IAI segments and tracks instances more accurately and robustly even in fast moving or occluded scenes. 
\input{Figures/fig8}
